# Supplementary material for: Linear Runlength-Limited Subcodes of Reed-Muller Codes and Coding Schemes for Input-Constrained BMS Channels
Source: arXiv:2205.04153 source file (2022-08-04)
Supplement: Supplementary file 2 [file appendix.tex]

In this section, we shall prove Lemma \ref{lemma:domain}.

\begin{proof}
	Consider a node $\mathbf{q} = (w_{0},\ldots,w_{d-1})\in \mathscr{V}_{\text{DB}}^{(d)}$ with accompanying vector $\boldsymbol{\beta}$. From equation \eqref{eq:theta_even} , we obtain that
	\begin{equation*}
	\theta_\mathbf{q}(d) = 1-a\sum_{s: w_s=?}\left(\frac{1}{1-a}\right)^{\beta_s}.
	\end{equation*}
	Let us define by $n_0$, the number of times a $0$ occurs in the $d$-tuple representation of $\mathbf{q}$, i.e., $n_0:=|\{s:w_s=0\}|$. Likewise, we define $n_?:=|\{s:w_s=\ ?\}|$. Now, the following sequence of inequalities holds:
	\begin{align*}
	\sum_{s: w_s=?}\left(\frac{1}{1-a}\right)^{\beta_s} &\leq n_? \left(\frac{1}{1-a}\right)^{n_0}\\
	&\leq n_? \left(1+\frac{1}{d}\right)^{n_0},
	\end{align*}
	where the last equality holds since $a\in [0,\frac{1}{d+1}]$, and, hence, $\frac{1}{\bar{a}}\in [1,1+\frac{1}{d}]$. Now, since $n_0 = d-n_?$, it follows that
	
	\begin{align*}
	\sum_{s: w_s=?}\left(\frac{1}{1-a}\right)^{\beta_s} &\leq n_? \left(1+\frac{1}{d}\right)^{d-n_?}\\
	&= n_?\left(1+\frac{1}{d}\right)^{d}\left(\frac{d}{d+1}\right)^{n_?}\\
	&\leq d\left(1+\frac{1}{d}\right)^{d}\left(\frac{d}{d+1}\right)^d\\
	&=d,
	\end{align*}
	where the last inequality follows from the fact that the function $g(u) := u\left(\frac{d}{d+1}\right)^u$ is increasing in the interval $[0,d]$.
	
	Hence, for $a\in [0,\frac{1}{d+1}]$, we have that 
	\begin{align*}
	\theta_\mathbf{q}(d)-a &\geq 1-a-ad\\
	&=1-a(d+1)\\
	&\geq 0,
	\end{align*}
	and, therefore, $a_\mathbf{q} = \frac{a}{\theta_\mathbf{q}(d)}\in [0,1]$.
	 
\end{proof}
