# Supplementary material for: Linear Runlength-Limited Subcodes of Reed-Muller Codes and Coding Schemes for Input-Constrained BMS Channels
Source: arXiv:2205.04153 source file (2022-08-04)
Supplement: Supplementary file 3 [file appendixb.tex]

The proof of equation \eqref{eq:append} is achieved by showing that 
\begin{equation}
	\label{eq:app1}
\Biggl|{m-t\choose \leq r_m}-{m-t\choose \leq r_{m-t}}\Biggr| = o(2^{m}),
\end{equation} 
for any fixed constant $t\in \mathbb{N}$. Modulo this fact, it holds that:
\begin{align*}
	\lim_{m\to \infty} \frac{{m-1 \choose \leq v_m}+{m-2\choose \leq v_m}}{2^m} &= \lim_{m\to \infty} \frac{{m-1 \choose \leq v_{m-1}}+{m-2\choose \leq v_{m-2}}}{2^m}\\
	&= \frac{1}{2}\cdot \lim_{m\to \infty} \frac{{m-1 \choose \leq v_{m-1}}}{2^{m-1}}+\frac{1}{4}\cdot \lim_{m\to \infty} \frac{{m-2 \choose \leq v_{m-2}}}{2^{m-2}}\\
	&= \frac{3R}{4},
\end{align*}
where the last equality holds since we assume that the sequence of codes $\{\hat{\mathcal{C}}_m = \text{RM}(m,v_m)\}$ achieves a rate $R\in (0,0.5)$ over the unconstrained BEC.

We shall now prove equation \eqref{eq:app1}. To this end, we use the following observation in \cite{kud3}, stated as Proposition \ref{prop:append}.
\begin{proposition}
	\label{prop:append}
	Consider a sequence of RM codes $\{\text{RM}(m,v_m)\}$ achieving a rate $R\in (0,1)$ over the unconstrained BEC. It is then true that
	\[
	v_m\in \left(\frac{m}{2}-\frac{m^{1/2+\beta}}{4},\frac{m}{2}+\frac{m^{1/2+\beta}}{4}\right),
	\]
	for any $\beta>0$.
\end{proposition}
Clearly, if $R\in (0,0.5)$, as in our case of interest, it is true that $v_m<\frac{m-t}{2}$, for any constant $t\in \mathbb{N}$, for $m$ large enough. Now, fix $\beta<1/6$. We then obtain the following set of inequalities for large enough $m$:
\begin{align*}
	\Biggl|{m-t\choose \leq r_m}-{m-t\choose \leq r_{m-t}}\Biggr| &\leq |v_m - v_{m-t}|\cdot {m-t \choose \min\{\frac{m-t}{2},v_m\}}\\
	&\stackrel{(a)}{=}|v_m - v_{m-t}|\cdot {m-t \choose v_m}\\
	&\stackrel{(b)}{\leq} m^{1/2+\beta}\cdot {m-t \choose \frac{m-t}{2}}\cdot e^{-\frac{m^{2\beta}}{2}},
\end{align*}
where 
\begin{enumerate}[label = (\alph*)]
	\item follows from the fact that $R<0.5$, and
	\item holds due to the identity (see, for example, \cite[Chap. 5, equation (5.42)]{asymp}) that for any $n$ large enough and for $k = \frac{n}{2}+\frac{c(n)\sqrt{n}}{2}$, with $c(n) = o(n^{1/6})$, it follows that
	\[
	{n\choose k}\sim {n\choose n/2}\cdot e^{-c(n)^2/2},
	\]
	where the symbol `$\sim$' is used to mean ``grows as''.
\end{enumerate}
From inequality (b) above, and from the following simple fact obtained by an application of Stirling's inequality (see, again, \cite[Chap. 5, equation (5.38)]{asymp})):
\[
{n\choose n/2}\sim \sqrt{\frac{2}{\pi n}}2^n,
\]
we get that for $\beta<1/6$, $c>0$, and $m$ large enough:
\begin{align*}
	{\Bigl|{m-t\choose \leq r_m}-{m-t\choose \leq r_{m-t}}\Bigr|}&\leq 2^m\cdot c m^\beta\cdot e^{-\frac{m^{2\beta}}{2}}\\
	&= o(2^m).
	%&\xrightarrow[m\to \infty]{} 0,
\end{align*}
